# Supplementary material for: CLIP-Embed-KD: Computationally Efficient Knowledge Distillation Using Embeddings as Teachers
Source: arXiv:2404.06170 source file (2024-04-09)
Supplement: Supplementary file 1 [file X_suppl.tex]

\clearpage
\setcounter{page}{1}
\maketitlesupplementary
\label{sec:supplementary}

\begin{table}[]
\centering
\begin{tabular}{c|c|c|c|c|c}
\textbf{Teacher} & \textbf{Layers} & \textbf{Patch size} & \textbf{Embed dim} & \textbf{Heads} & \multicolumn{1}{l}{\textbf{MLP}} \\ \hline
Base & 12 & 16 / 32 & 768 & 12 & 3072 \\
Large & 24 & 16 / 32 & 1024 & 16 & 4096                           
\end{tabular}
\caption{Architecture specification of the teacher models.}
\label{tab:teacher_arch}
\end{table}

%\begin{figure}[!t]
%\centering
%\includegraphics[width=0.48\textwidth]{imgs/Clip-teacher-KD-%algo.png}
%\caption{Pseudocode showing the CLIP-Teacher-KD algorithm.}
%\label{fig:clip-teacher-kd-algo}
%\end{figure}

%\begin{figure}[!t]
%\centering
%\includegraphics[width=0.48\textwidth]{imgs/CLIP-embed-KD-%algo.png}
%\caption{Pseudocode showing the CLIP-Embed-KD algorithm.}
%\label{fig:clip-embed-kd-algo}
%\end{figure}
